# Supplementary material for: Differentiable Meta Multigraph Search with Partial Message Propagation on Heterogeneous Information Networks
Source: arXiv:2211.14752 source file (2022-11-27)
Supplement: Supplementary file 1 [file robust_step_appendix.tex]

\begin{figure}[!t]
\centering
\subfigure[ACM]{\includegraphics[width=0.48\linewidth]{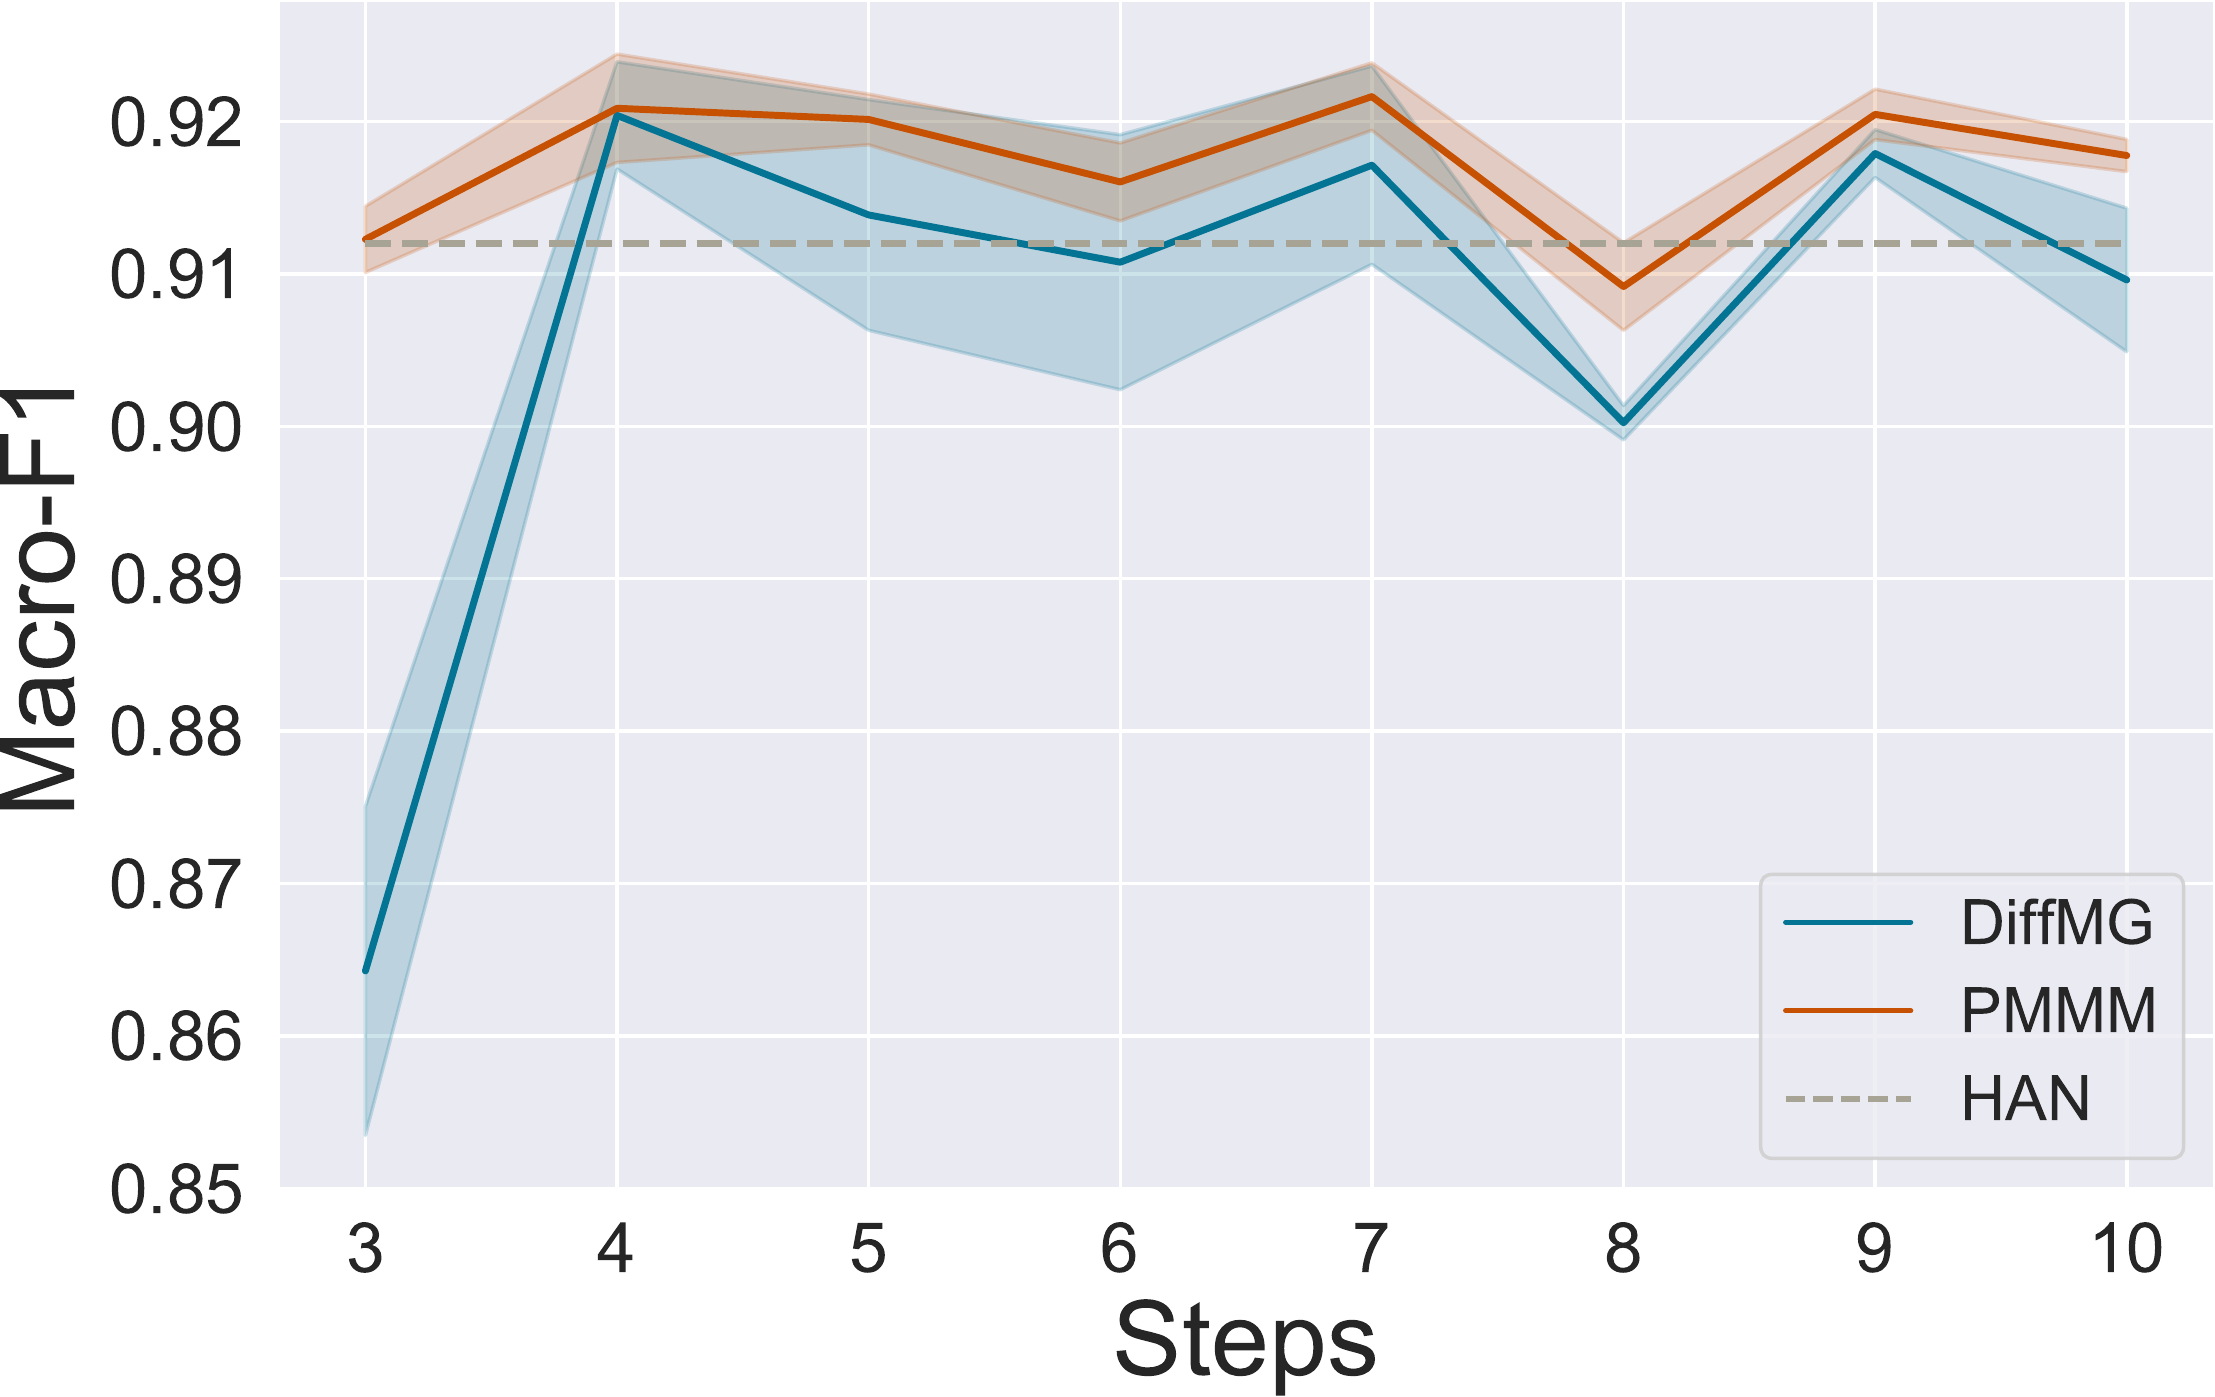}}
\hspace{0.1em}
\subfigure[IMDB]{\includegraphics[width=0.48\linewidth]{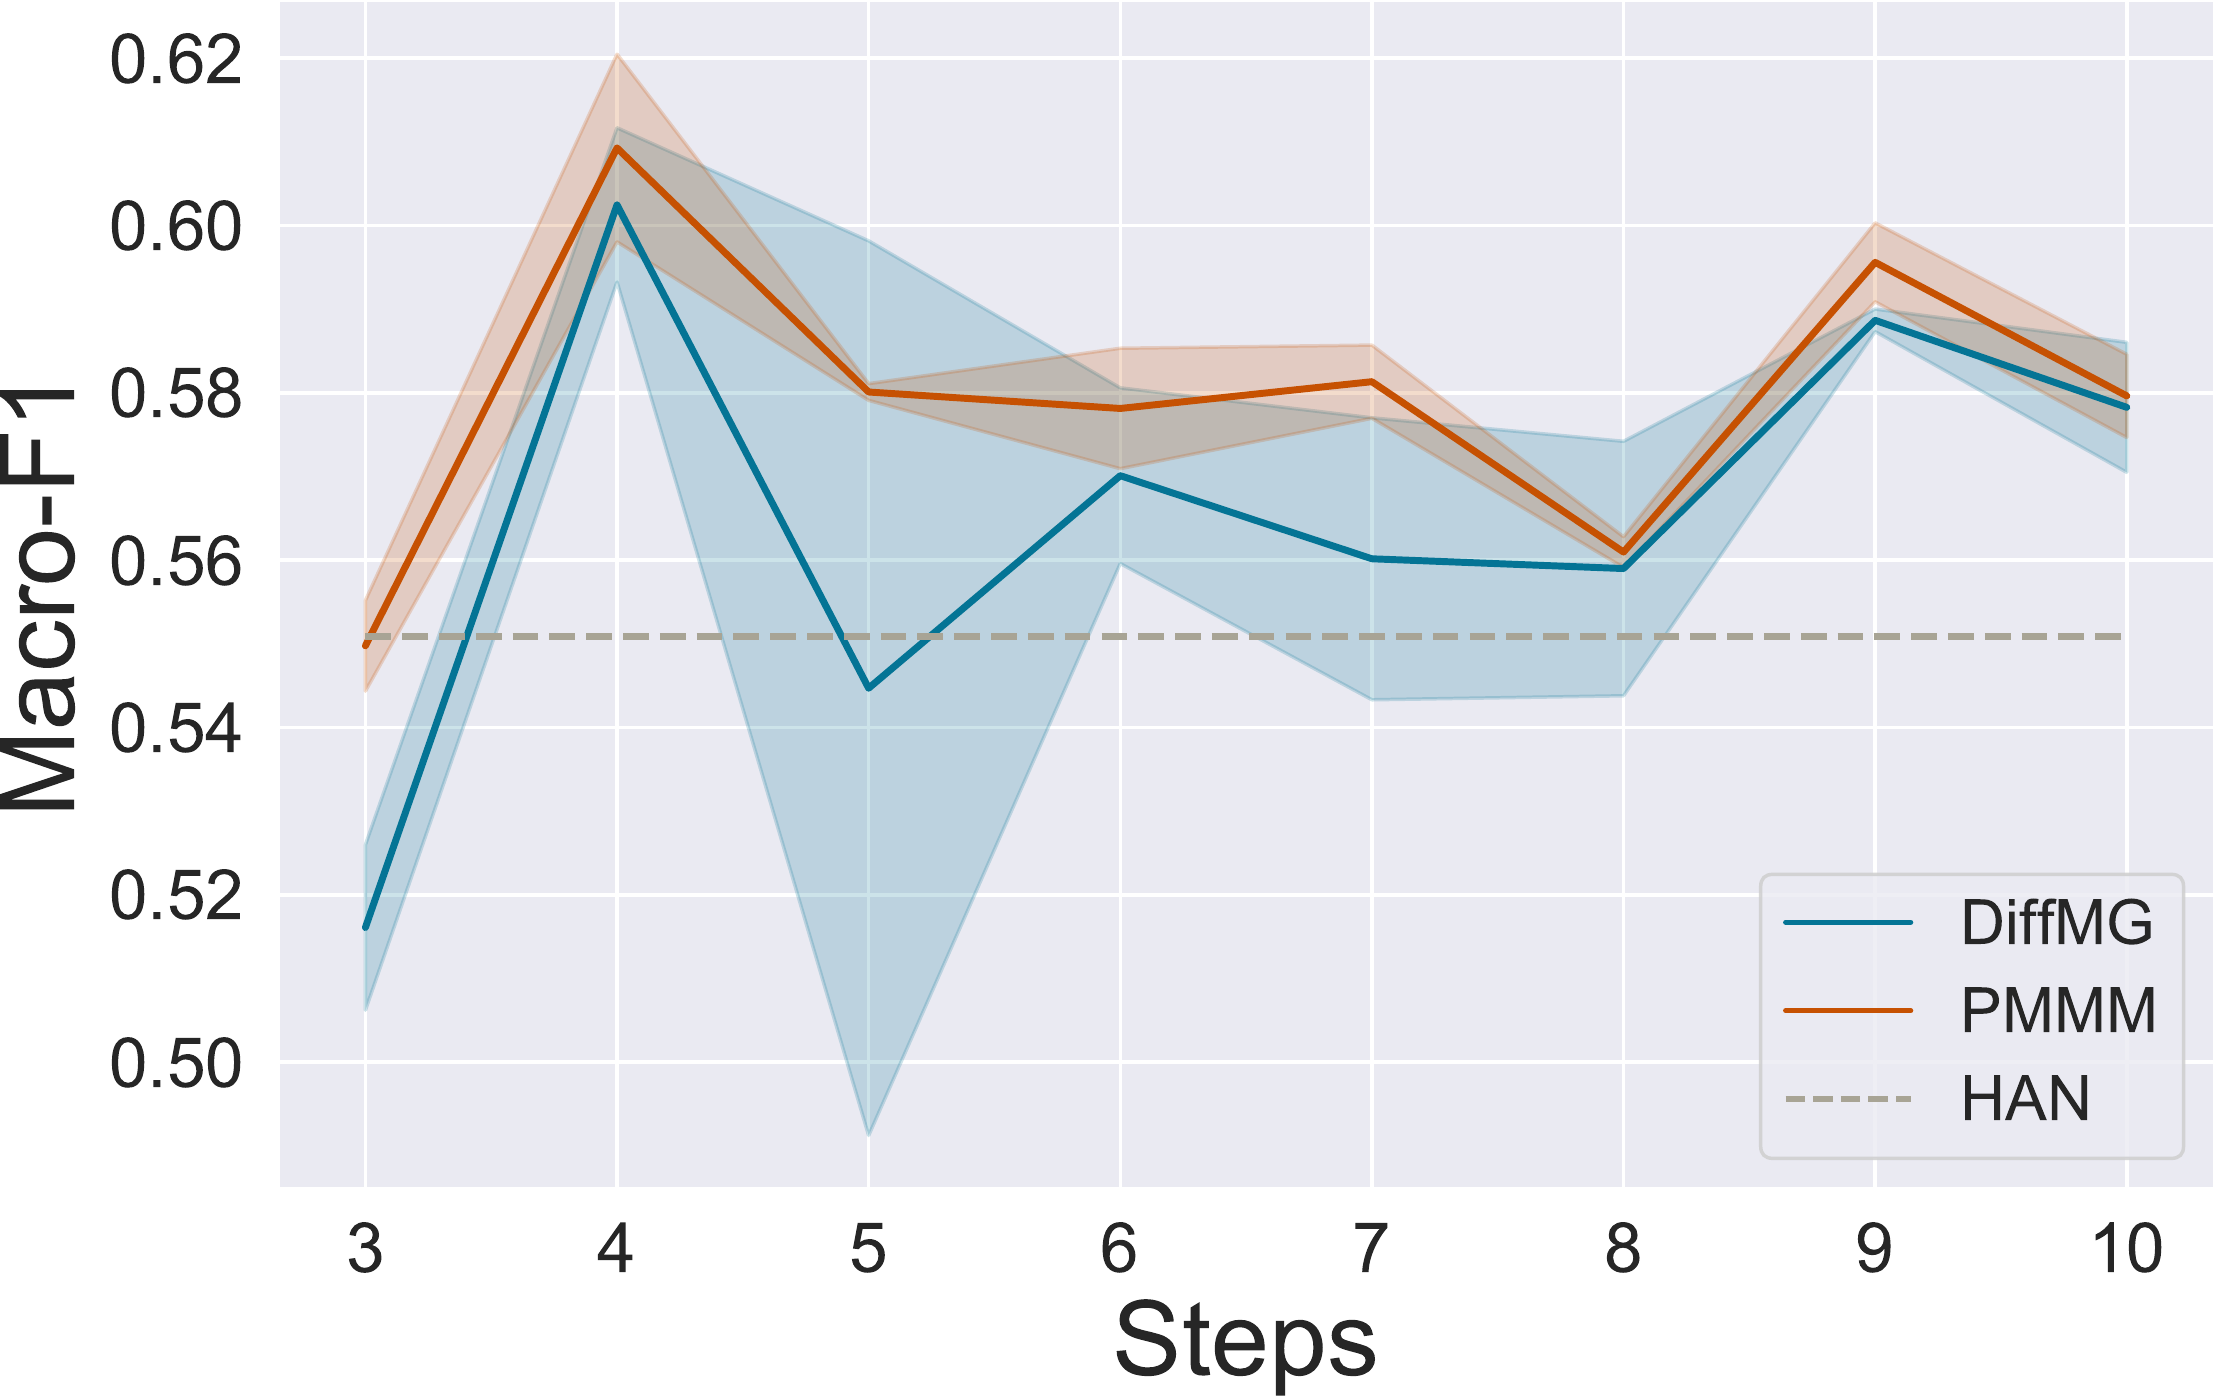}}
\\
\subfigure[Amazon]{\includegraphics[width=0.48\linewidth]{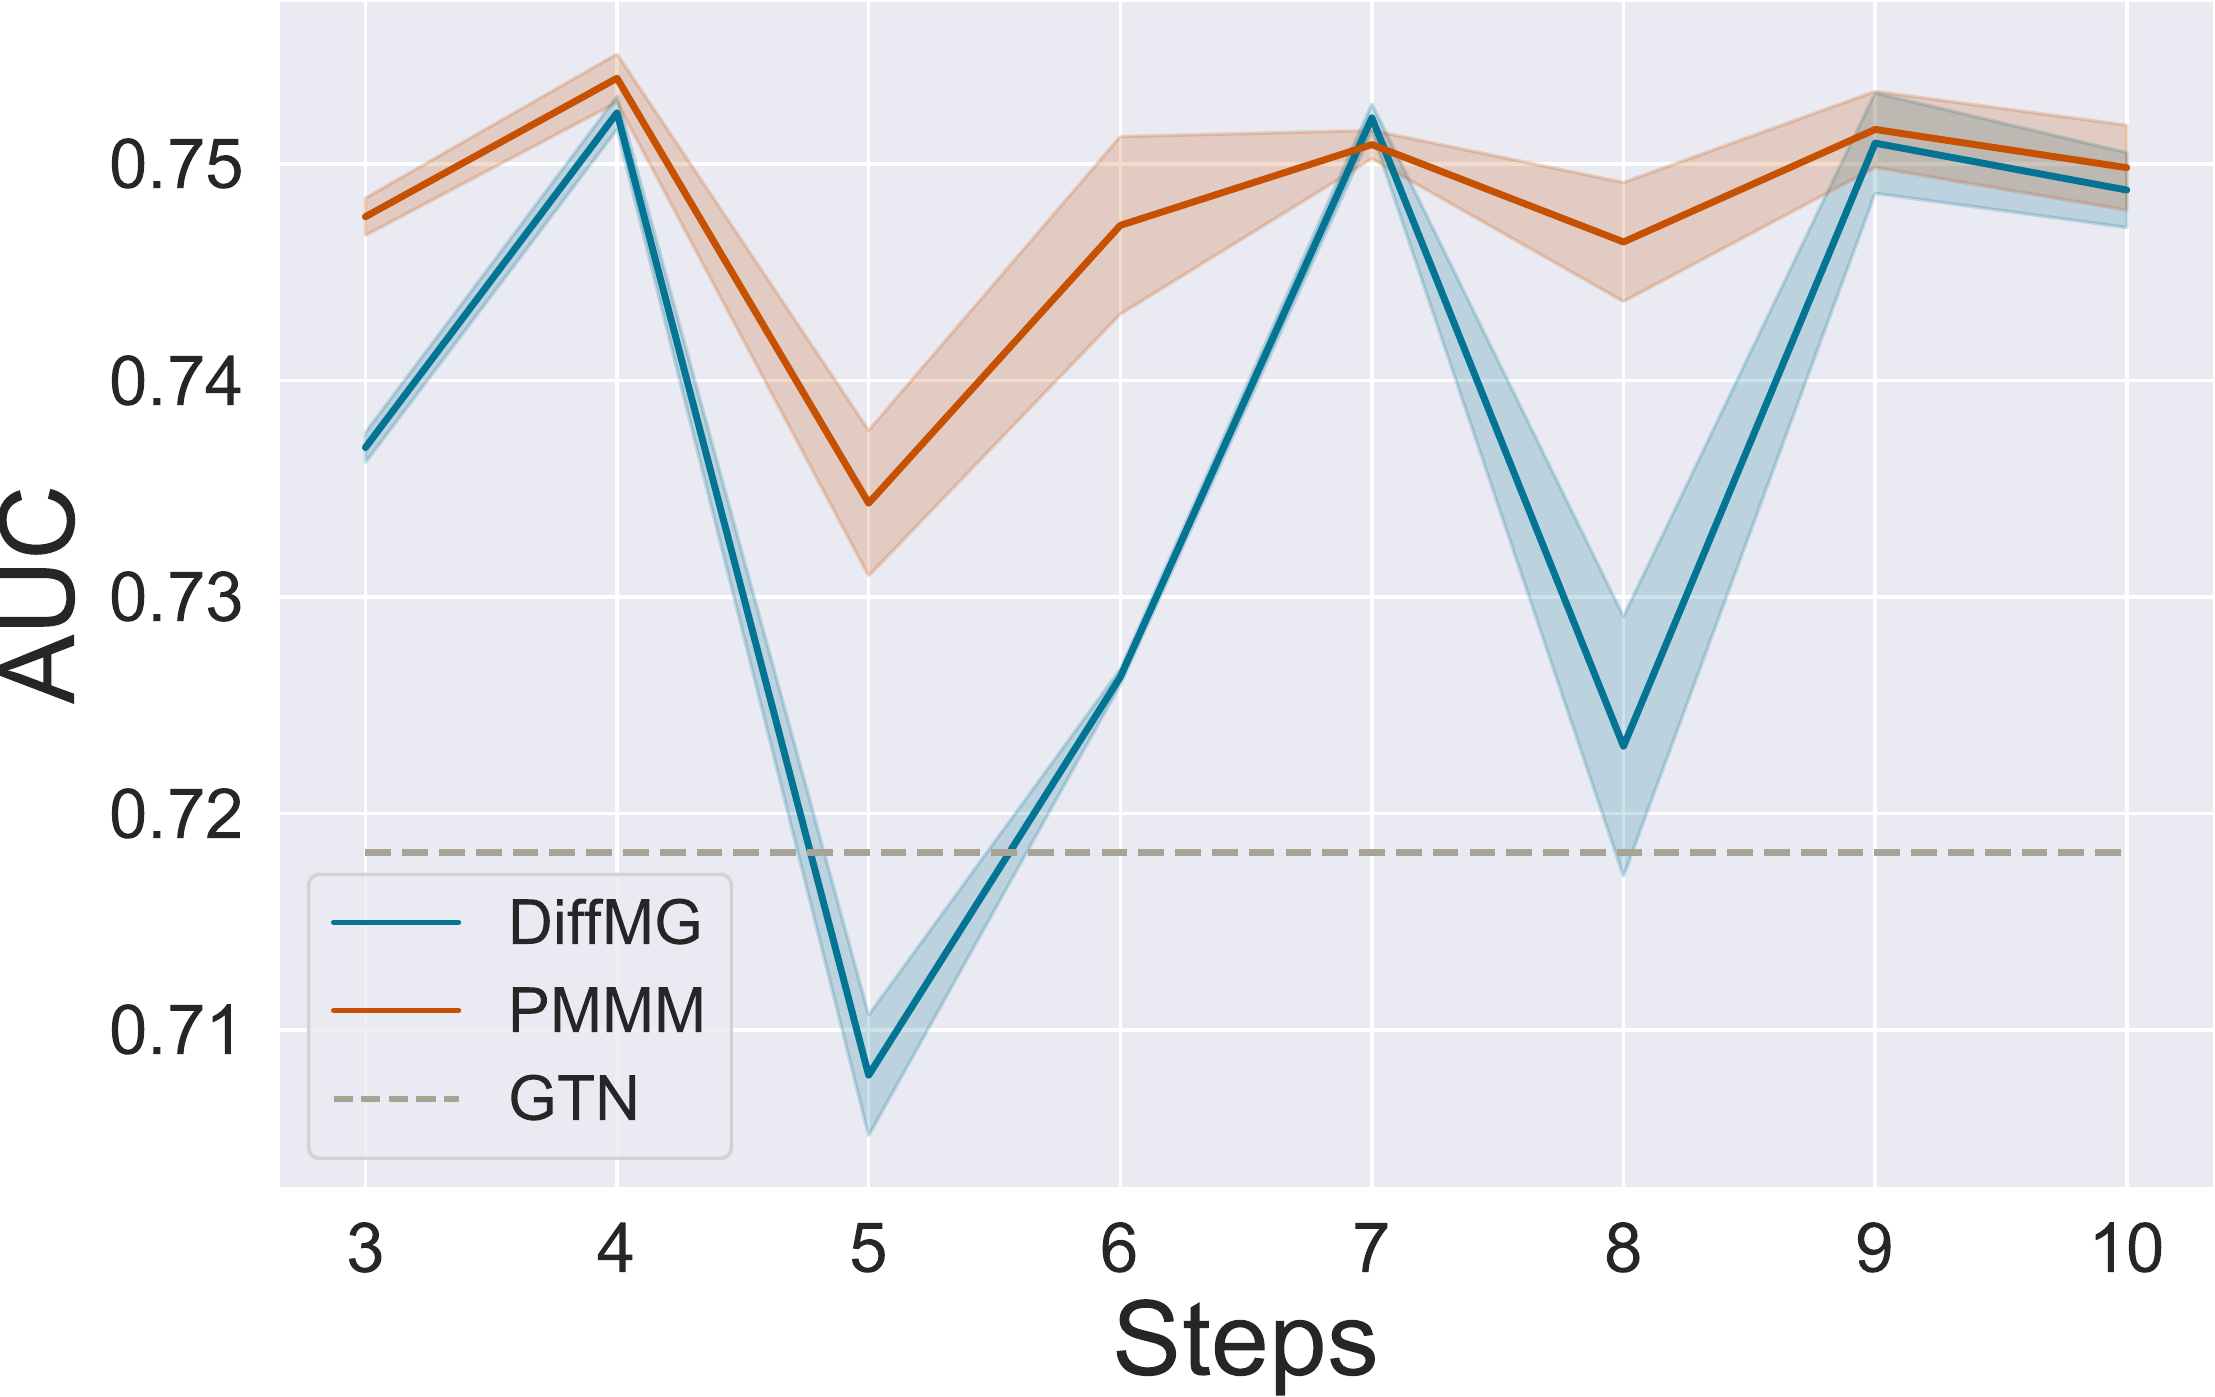}}
\hspace{0.1em}
\subfigure[Douban]{\includegraphics[width=0.48\linewidth]{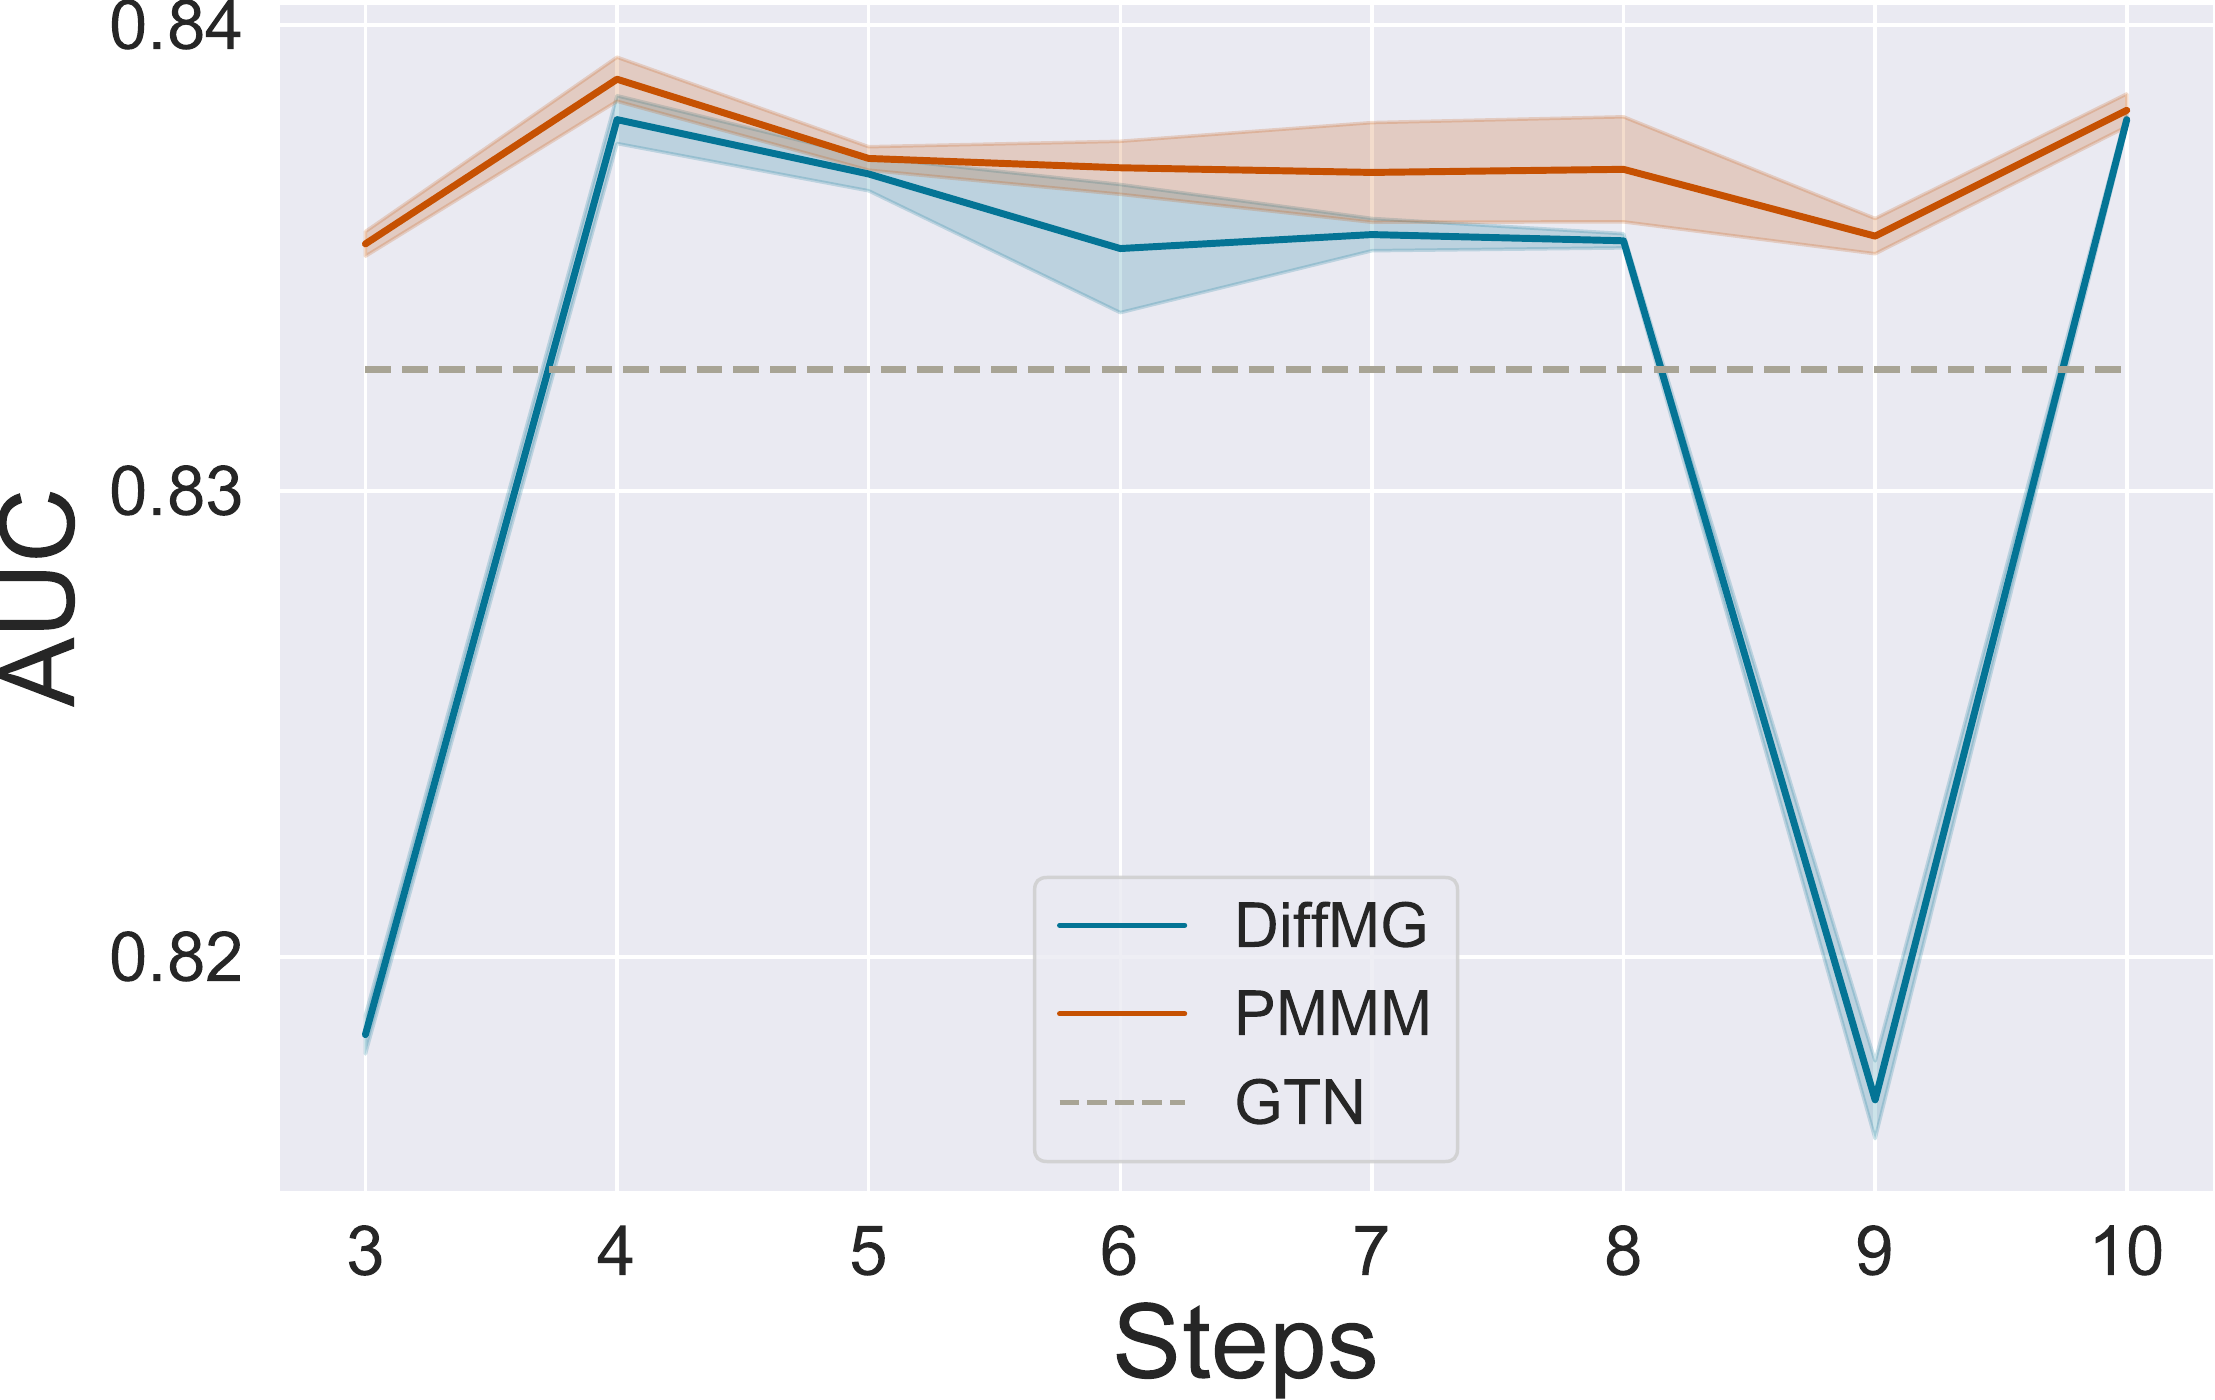}}
\caption{Performance on different search steps. (best viewed in color). 
(a) Macro F1 scores on ACM.
(b) Macro F1 scores on IMDB.
(c) AUC on Amazon.
(d) AUC on Douban Movie.
%The first three are node classification tasks, and the last three are recommendation tasks.
}

\label{fig:step_appendix}
\end{figure}

% \begin{figure}[!t]
% \centering
% \subfigure[DBLP]{\includegraphics[width=0.48\linewidth]{fig/DBLP_steps.pdf}}
% \hspace{0.1em}
% \subfigure[Yelp]{\includegraphics[width=0.48\linewidth]{fig/Yelp_steps.pdf}}

% \caption{Performance on different search steps. (best viewed in color). 
% (a) Macro F1 scores on DBLP.
% (b) AUC on Yelp. }
% \vspace{-0.5em}
% \label{fig:step}
% \end{figure}
